# Supplementary material for: The Heisenberg-RIXS instrument at the European XFEL
Source: arXiv:2403.08461 ancillary file (2024-03-13)
Supplement: Supplementary file 1 [file Heisenberg-RIXS_Instrument_SUPPLEMENT.pdf]

Supplemental Material for:

# The Heisenberg-RIXS instrument at the European XFEL

Justine Schlappa,[a,*] Giacomo Ghiringhelli,[b,c,#] Benjamin E. Van Kuiken,[a] Martin Teichmann,[a] Piter S. Miedema,[a] Jan Torben Delitz,[a] Natalia Gerasimova,[a] Serguei Molodtsov,[a] Luigi Adriano,[a] Bernard Baranasic,[a] Carsten Broers,[a] Robert Carley,[a] Patrick Gessler,[a] Nahid Ghodrati,[a] David Hickin,[a] Le Phuong Hoang,[a] Manuel Izquierdo,[a] Laurent Mercadier,[a] Giuseppe Mercurio,[a] Sergii Parchenko,[a] Marijan Stupar,[a] Zhong Yin,[a] Leonardo Martinelli,[b] Giacomo Merzoni,[a,b] Ying Ying Peng,[b,d] Torben Reuss,[e] Sreeju Sreekantan Nair Lalithambika,[e,f] Simone Techert,[e,f,†] Tim Laarmann,[e,g,◦] Simo Huotari,[h] Christian Schroeter,[i] Burkhard Langer,[i] Tatjana Giessel,[i] Robby Buechner,[j] Jana Buchheim,[j] Vinicius Vaz da Cruz,[j] Sebastian Eckert,[j] Grzegorz Gwalt,[j] Chun-Yu Liu,[j,k] Frank Siewert,[j] Christian Sohrt,[j] Christian Weniger,[j] Annette Pietzsch,[j] Stefan Neppl,[k,l] Friedmar Senf,[k] Andreas Scherz[a,%] and Alexander Föhlisch[j,k,$]

*[a]European XFEL, Holzkoppel 4, Schenefeld, 22869, Germany, [b]Dipartimento di Fisica, Politecnico di Milano, piazza Leonardo da Vinci 32, I-20133 Milano, Italy, [c]CNR-SPIN, Dipartimento di Fisica, Politecnico di Milano, I-20133 Milano, Italy, [d]Present address: International Center for Quantum Materials, School of Physics, Peking University, Beijing 100871, China, [e]Deutsches Elektronen-Synchrotron DESY, Notkestraße 85, 22607 Hamburg, Germany, [f]Institute of X-ray Physics, Goettingen University, Friedrich Hund Platz 1, 37077 Goettingen, Germany, [g]The Hamburg Centre for Ultrafast Imaging CUI, Luruper Chaussee 149, 22761 Hamburg, Germany, [h]Department of Physics, University of Helsinki, P.O. Box 64, FI-00014 Helsinki, Finland, [i]BESTEC GmbH, Am Studio 2b, 12489 Berlin, Germany, [j]Institute Methods and Instrumentation for Synchrotron Radiation Research, Helmholtz-Zentrum Berlin für Materialien und Energie GmbH, Albert-Einstein-Straße 15, 12489 Berlin, Germany, [k]University of Potsdam, Institute of Physics and Astronomy, Karl-Liebknecht-Straße 24/25, 14476 Potsdam, Germany, [l]Present address: Paul Scherrer Institut, Forschungsstrasse 111, 5232 Villigen PSI, Switzerland,*

*[*] justine.schlappa@xfel.eu, [#] giacomo.ghiringhelli@polimi.it, [%] andreas.scherz@xfel.eu, [†] simone.techert@desy.de, [◦] tim.laarmann@desy.de, and [$] alexander.foehlisch@helmholtz-berlin.de*

a)

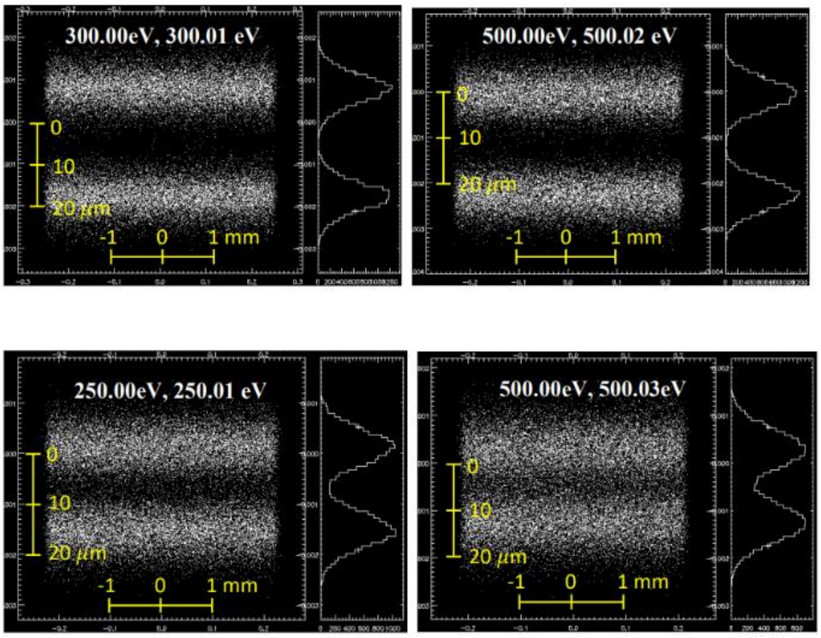


b)

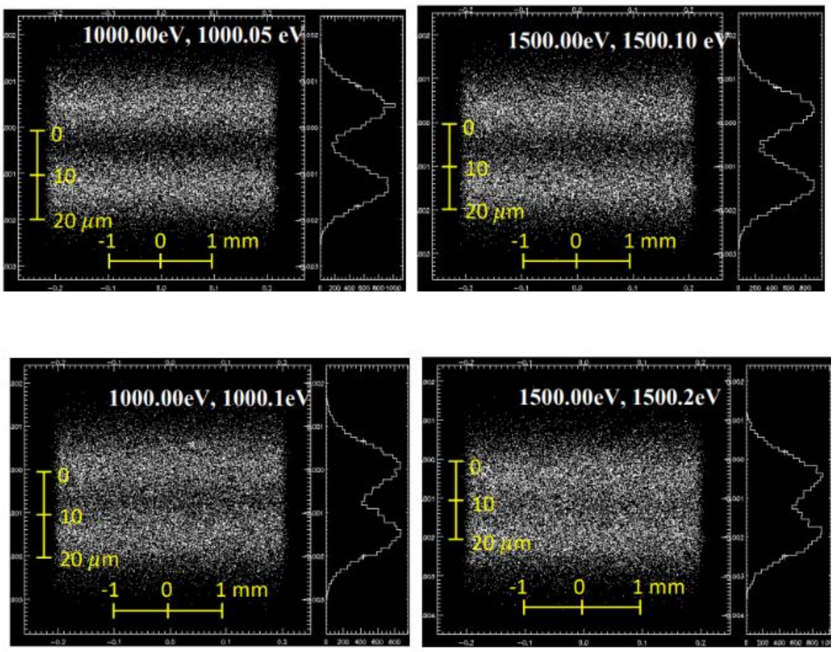


Fig. S1: Ray-tracing simulations for hRIXS spectrometer for photon energies of 250 eV - 500 eV (a) and 1,000 eV -1,500 eV (b) made with Shadows. Top figures show results for HRG (1,000 l/mm grating) and bottom figures for HTG (3,000 l/mm), respectively. The source has Gaussian spatial distribution with FWHM $S_1$ = 5 µm and angular divergence of 1 mrad in both directions. The spatial intensity distribution on the surface of the detector of two monochromatic lines of energy indicating at the top of each panel are shown.

a)

Min. Abstand Detektorkammer-
Gitterkammer: 2196
(1500 eV / 1000 l/mm / 88,7°: 2196)
Min Balglänge: 2196 - 100 mm

Max. Abstand Detektorkammer-
Gitterkammer: 3422
(250 eV / 3000 l/mm / 88,6°: 3422)
Max Balglänge: 3422 + 100 mm

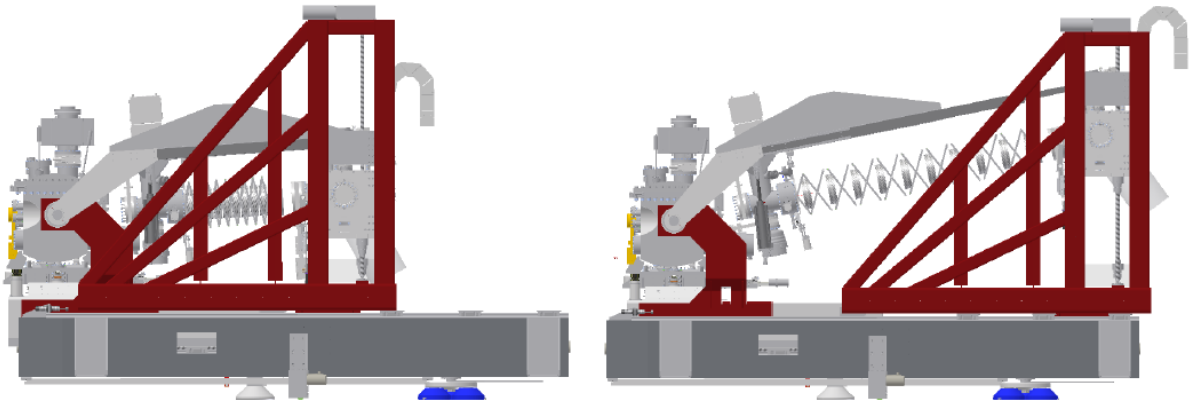

b)

Legend: no access possible (red); r1 < 1300 mm (orange); best resolution (blue); best transmission (green)

**3000L/mm**
**r1 (entrance arm)**

| | 88° | 88,1° | 88,2° | 88,3° | 88,4° | 88,5° | 88,6° | 88,7° | 88,8° | 88,9° | 89° |
|---|---|---|---|---|---|---|---|---|---|---|---|
| 250 eV | | | | | | | 1636 | 1505 | 1377 | 1251 | 1128 |
| 300 eV | | | | | | 1609 | 1486 | 1365 | 1248 | 1132 | 1019 |
| 400 eV | | | | 1716 | 1598 | 1481 | 1368 | 1256 | 1148 | 1041 | 936 |
| 500 eV | | | 1779 | 1661 | 1546 | 1434 | 1323 | 1216 | 1110 | 1007 | 905 |
| 600 eV | | 1870 | 1752 | 1636 | 1523 | 1412 | 1304 | 1198 | 1094 | 992 | |
| 700 eV | | 1857 | 1740 | 1625 | 1513 | 1403 | 1295 | 1190 | 1086 | 985 | |
| 800 eV | | 1852 | 1736 | 1621 | 1509 | 1400 | 1292 | 1187 | 1084 | 983 | |
| 900 eV | 1970 | 1851 | 1735 | 1621 | 1509 | 1400 | 1292 | 1187 | 1084 | 983 | |
| 1000 eV | 1971 | 1853 | 1737 | 1623 | 1511 | 1401 | 1294 | 1188 | 1085 | 984 | |
| 1100 eV | 1975 | 1856 | 1740 | 1626 | 1514 | 1404 | 1296 | 1191 | 1088 | 986 | |
| 1200 eV | 1979 | 1860 | 1744 | 1630 | 1518 | 1408 | 1300 | 1194 | 1090 | 989 | |
| 1300 eV | 1983 | 1865 | 1748 | 1634 | 1522 | 1412 | 1304 | 1198 | 1094 | 992 | |
| 1400 eV | 1988 | 1870 | 1753 | 1639 | 1526 | 1416 | 1308 | 1201 | 1097 | 995 | |
| 1500 eV | 1993 | 1875 | 1758 | 1643 | 1531 | 1420 | 1312 | 1205 | 1101 | 998 | |

**1000L/mm**
**r1 (entrance arm)**

| | 88° | 88,1° | 88,2° | 88,3° | 88,4° | 88,5° | 88,6° | 88,7° | 88,8° | 88,9° | 89° |
|---|---|---|---|---|---|---|---|---|---|---|---|
| 250 eV | | | 1925 | 1794 | 1666 | 1541 | 1420 | 1301 | 1186 | 1073 | 963 |
| 300 eV | | 2046 | 1913 | 1783 | 1656 | 1533 | 1412 | 1294 | 1179 | 1067 | 958 |
| 400 eV | | 2044 | 1912 | 1783 | 1657 | 1534 | 1413 | 1296 | 1181 | 1068 | 959 |
| 500 eV | | 2054 | 1923 | 1793 | 1667 | 1543 | 1423 | 1304 | 1189 | 1076 | |
| 600 eV | 2202 | 2067 | 1935 | 1806 | 1679 | 1555 | 1434 | 1315 | 1199 | 1085 | |
| 700 eV | 2215 | 2081 | 1949 | 1819 | 1692 | 1567 | 1445 | 1326 | 1209 | | |
| 800 eV | 2227 | 2093 | 1961 | 1831 | 1704 | 1579 | 1456 | 1336 | 1218 | | |
| 900 eV | 2239 | 2105 | 1973 | 1843 | 1715 | 1590 | 1466 | 1346 | 1227 | | |
| 1000 eV | 2250 | 2116 | 1984 | 1854 | 1726 | 1600 | 1476 | 1355 | 1236 | | |
| 1100 eV | 2260 | 2126 | 1994 | 1863 | 1735 | 1609 | 1485 | 1363 | 1244 | | |
| 1200 eV | 2269 | 2135 | 2003 | 1872 | 1744 | 1618 | 1493 | 1371 | | | |
| 1300 eV | 2277 | 2143 | 2011 | 1881 | 1752 | 1626 | 1501 | 1378 | | | |
| 1400 eV | 2285 | 2151 | 2019 | 1889 | 1760 | 1633 | 1508 | 1385 | | | |
| 1500 eV | 2292 | 2158 | 2026 | 1896 | 1767 | 1640 | 1515 | 1392 | | | |

Fig. S2: Horizontal movement range for the hRIXS detector chamber (a) and grating chamber (b). The movement range gives a large working range for each photon energy, so that optimization either on energy resolution or on transmission is possible. The demands on the mechanical construction are high, e.g. the length of bellow connecting the grating and detector chamber can change from 2096 mm to 3522 mm (a).

a)

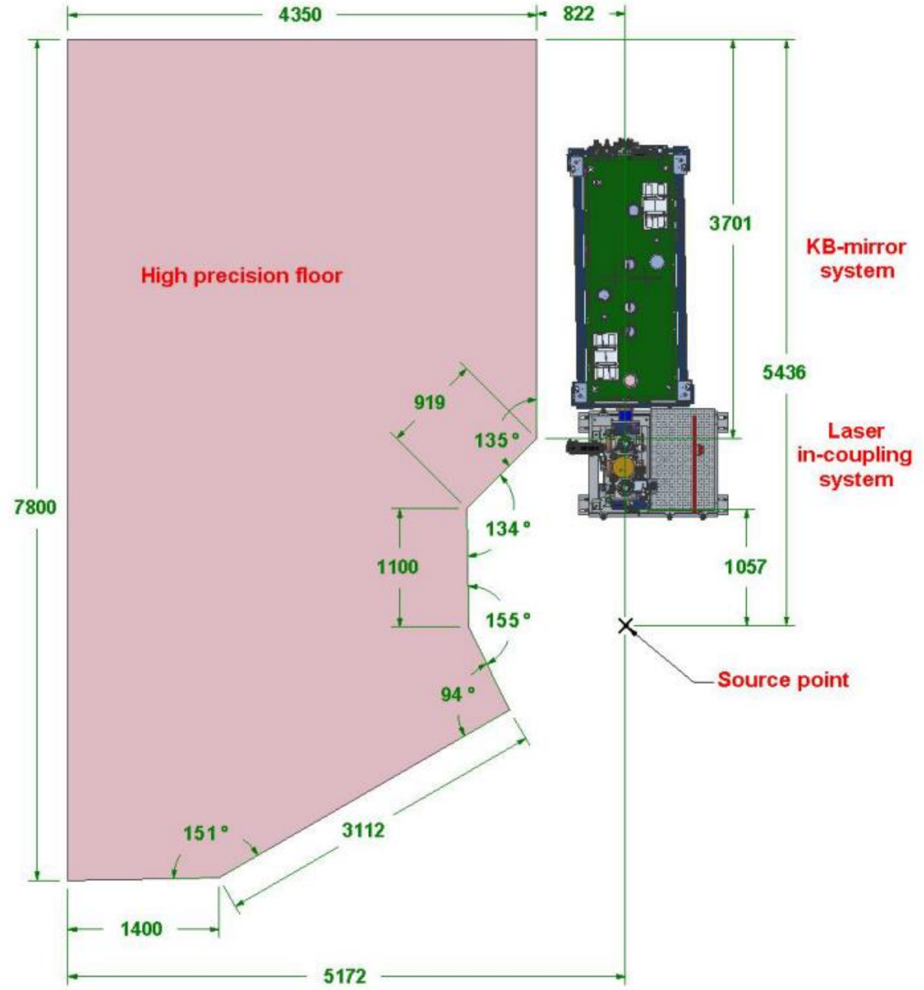


b)

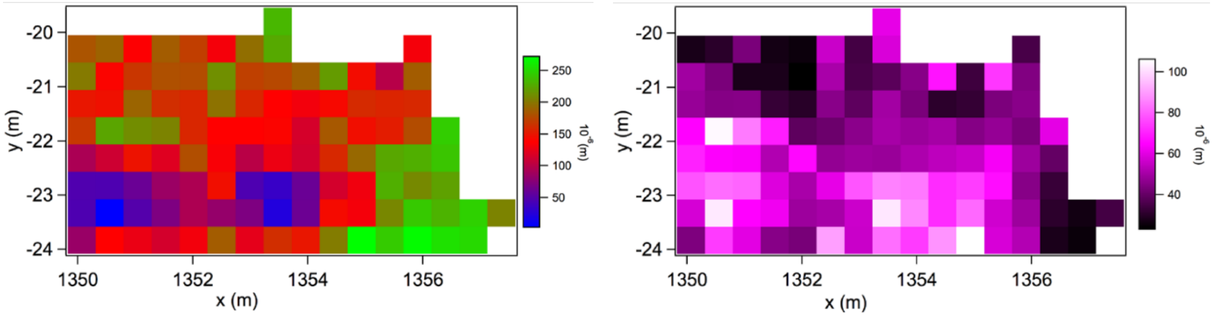


Fig. S3: Dimensions and location of the high-quality floor (HQF) inside the SCS hutch (a). The length along the beamline direction is about 7 m and perpendicular to the beamline around 4 m. The shape of the floor had to be adopted to the specific situation inside SCS hutch and leave enough space (next to the source point) for installation of rails for hRIXS rotation. Geodetic measurement results for height variation of the HQF (left) and planarity averaged over 1 m (right) (b). Results are shown in µm, the horizontal (vertical) axis refers to coordinates inside SCS hutch along (perpendicular to) the beamline. The maximum height variation over the entire HQF area is in the rage of 250 µm.

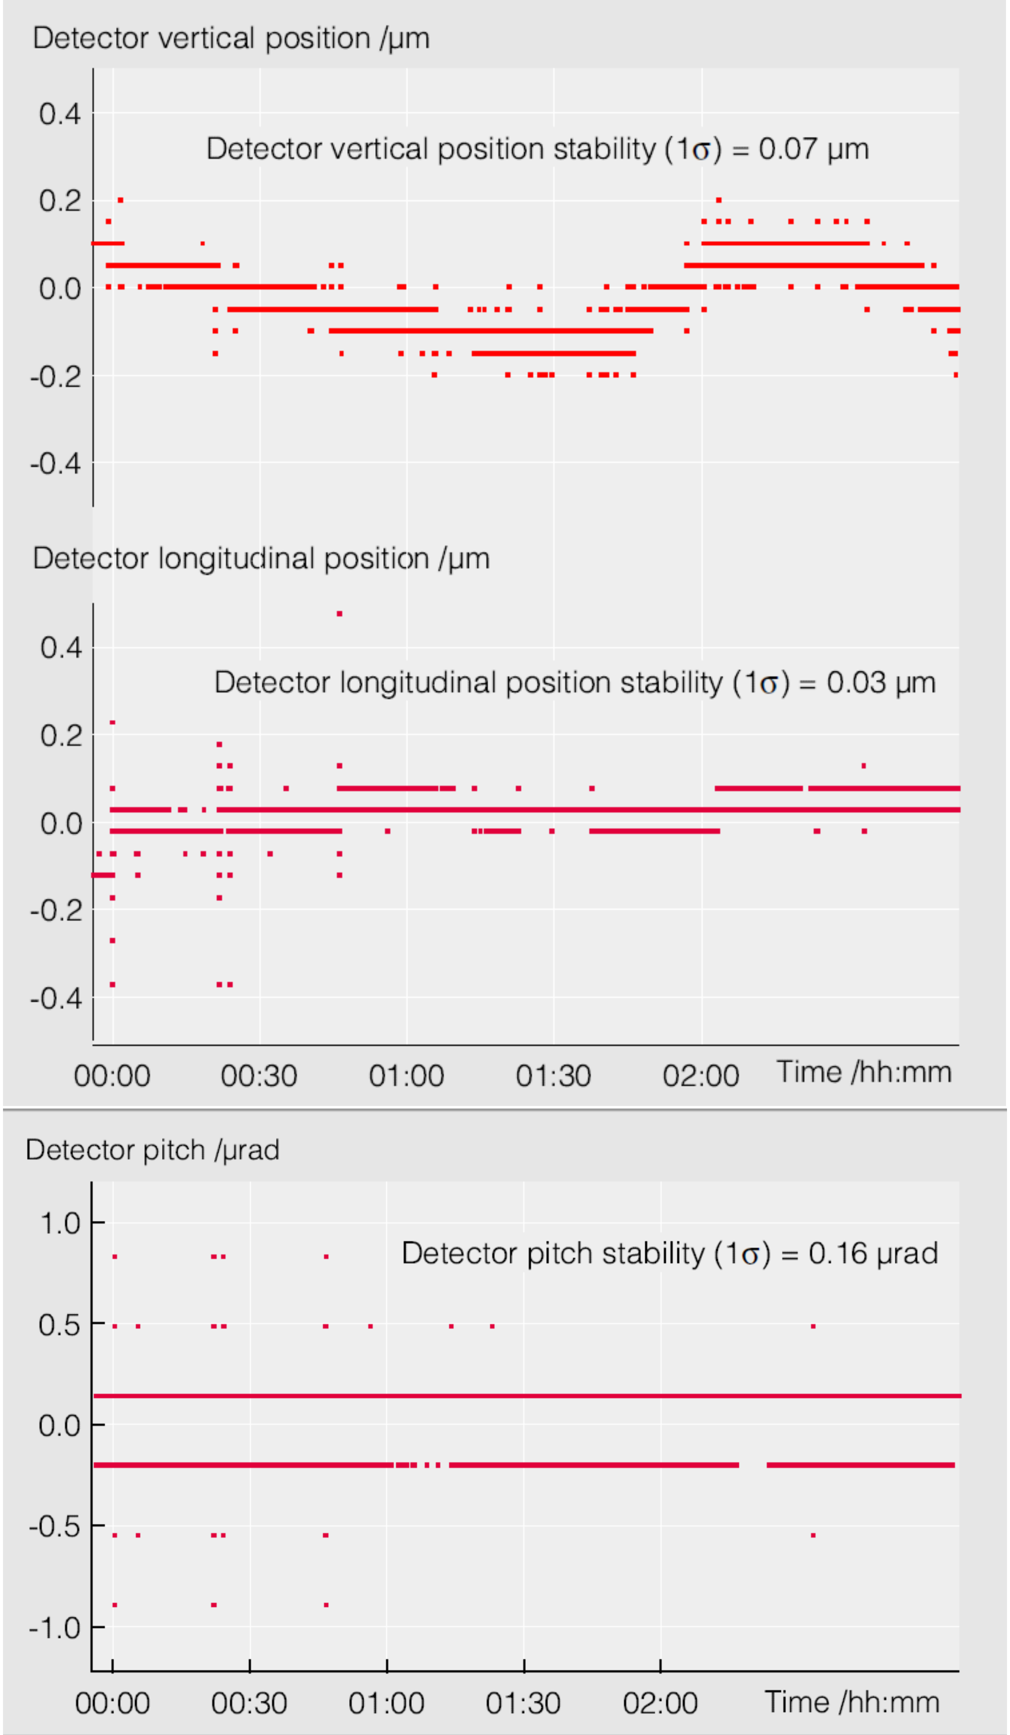


Fig. S4: Stability measurements for detector-chamber position after installation of the hRIXS spectrometer at the source point. Displayed is encoder data for detector height, distance and pitch, measured over duration of 3 h (the data is neither averaged or filtered).

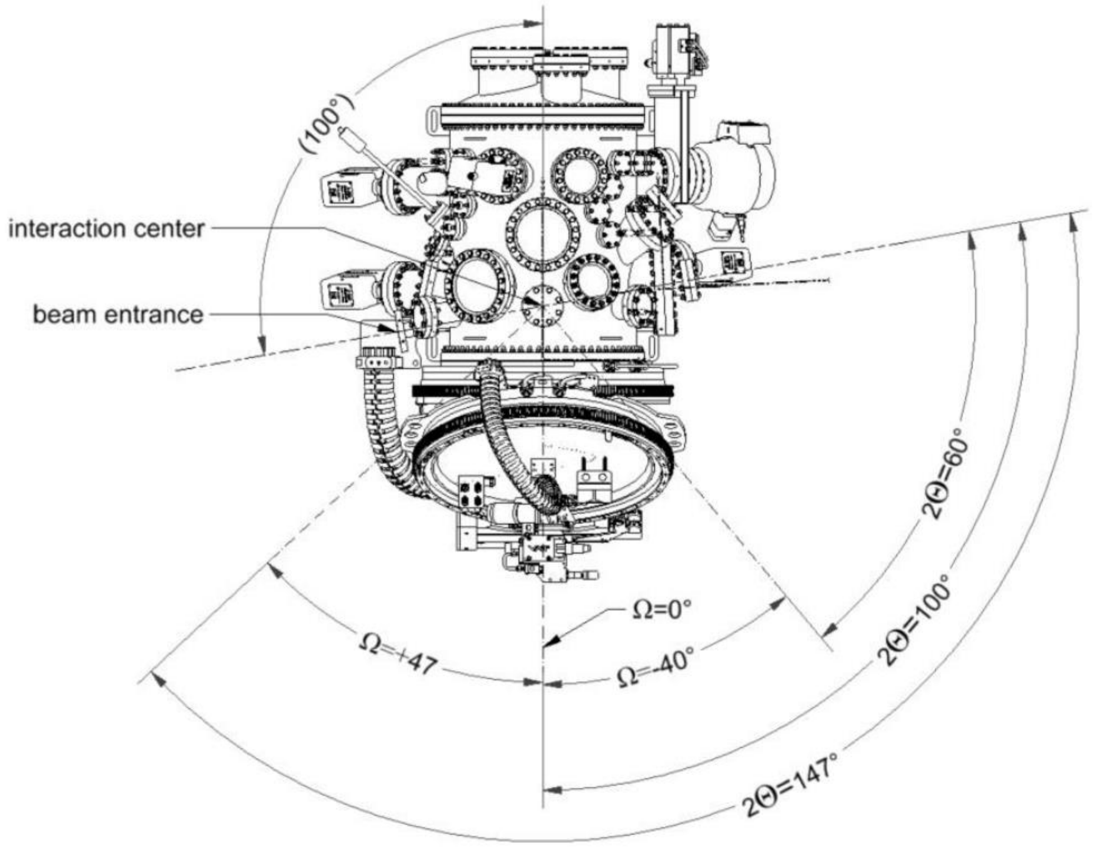


Fig. S5: Swivel range of the triple-rotating flange (TRF) of the XRD chamber. The vessel is oriented with an offset of 10° in respect to the FEL beam, in order to maximize the accessible TRF back-scattering angle (Two-theta of 147°). The minimum TRF forward-scattering angle is 60° in Two-Theta.

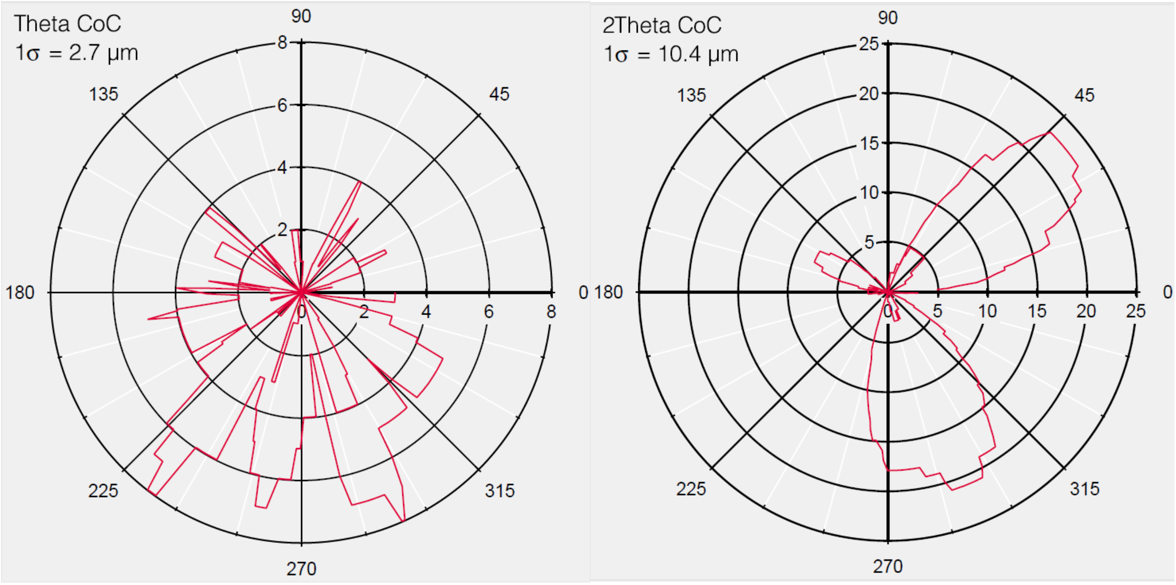


Fig. S6: Circle-of-confusion data (dial gauge signal) for sample Theta and detector Two-Theta rotation of the in-vacuum XRD diffractometer.

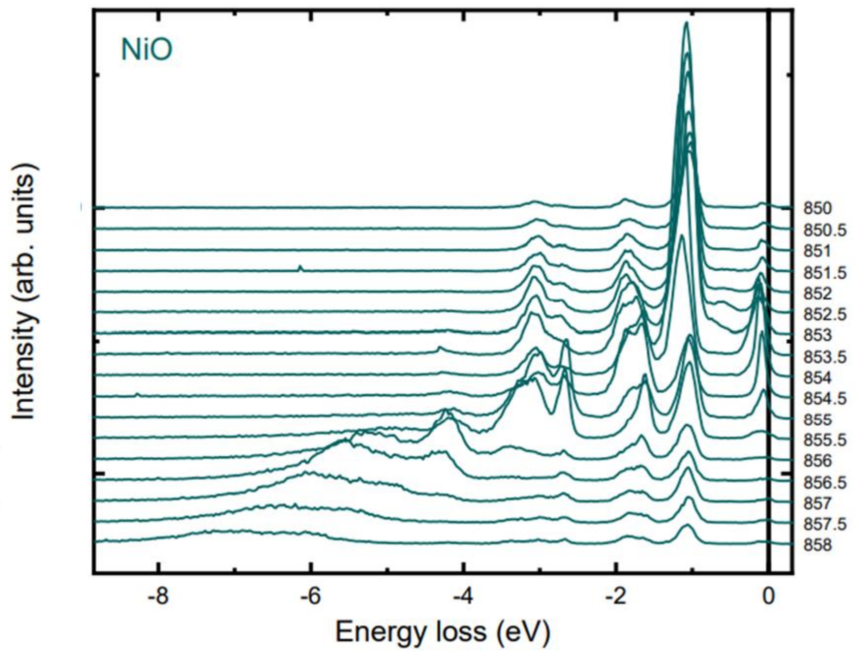


Fig. S7: RIXS data obtained from single-crystal NiO at room temperature across the Ni $L_3$ resonance. Acquisition time per spectrum was 60 s. Data was taken at 1.1 MHz repetition rate, 400 pulses per train and 100% transmission.
